# Supplementary material for: The ProtoDUNE-SP LArTPC Electronics Production, Commissioning, and Performance
Source: arXiv:2002.01782 source file (2020-04-30)
Supplement: Supplementary file 1 [file appendix.tex]

\section{Other Stuff}\label{sec:otherstuff}
